# Supplementary material for: Simulation of Vibronic Strong Coupling and Cavity-Modified Hydrogen Tunneling Dynamics
Source: arXiv:2506.18647 source file (2025-06-23)
Supplement: Supplementary file 1 [file SuppInfo.pdf]

# Supplementary Material:

## Simulation of Vibronic Strong Coupling and Cavity-Modified Hydrogen Tunneling Dynamics

Scott M. Garner<sup>1</sup>, Xiaosong Li<sup>2</sup>, and Sharon Hammes-Schiffer<sup>\*1</sup>

<sup>1</sup>Department of Chemistry, Princeton University, Princeton, NJ 08544, United  
States

<sup>2</sup>Department of Chemistry, University of Washington, Seattle, WA 98195,  
United States

\*Email: shs566@princeton.edu

June 23, 2025

### Contents

|                                           |    |
|-------------------------------------------|----|
| S1 Additional HeHHe <sup>+</sup> Analysis | S2 |
| S2 HCN Vibronic Strong Coupling           | S3 |

## S1 Additional HeHHe<sup>+</sup> Analysis

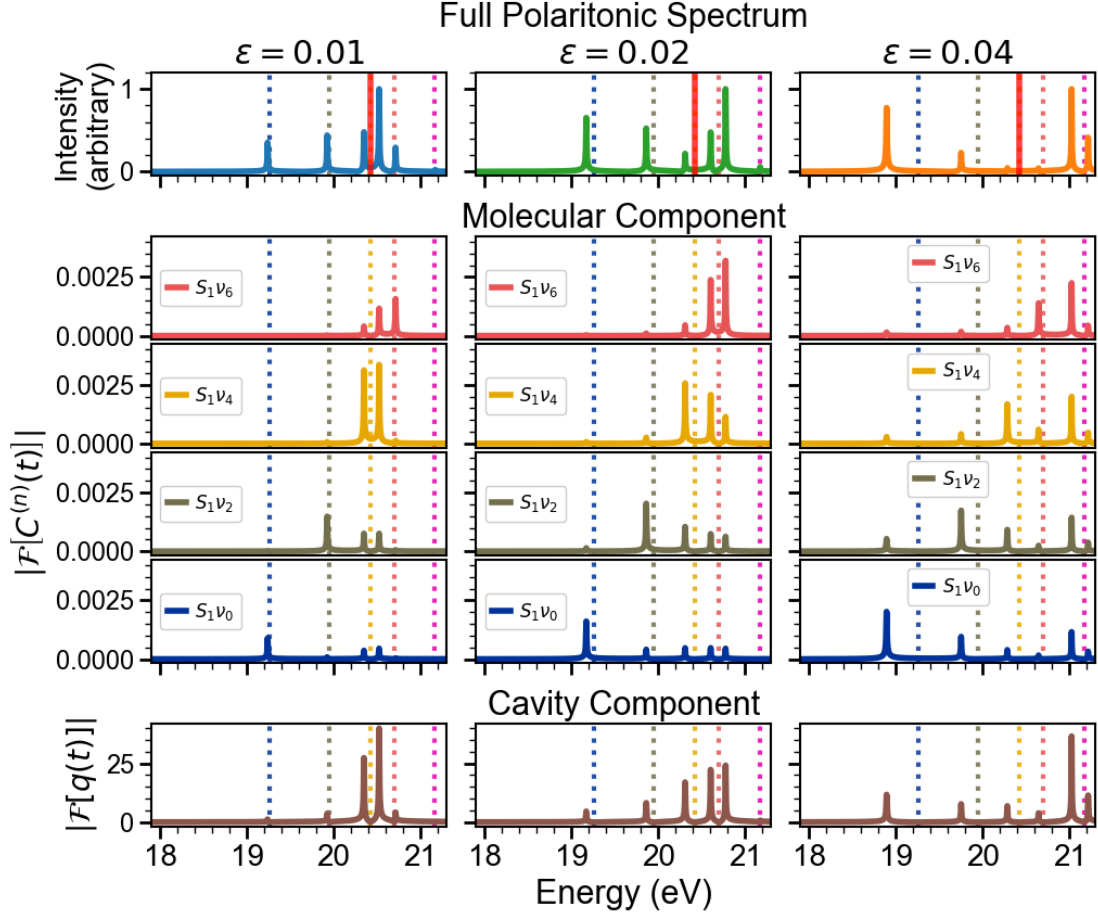

Figure S1: Top row: Semiclassical NEO-TDCI spectra of HeHHe<sup>+</sup> calculated with the cavity mode frequency tuned to the  $S_0\nu_0 \rightarrow S_1\nu_4$  transition (solid red lines) and the light-matter coupling constant indicated above each column. Middle set of plots: Fourier transforms of the projected coefficients of the relevant molecular vibronic states for the light-matter coupling constants indicated above each column. Bottom row: Fourier transforms of the classical cavity mode displacement coordinate. On all plots, the dotted vertical lines indicate the energies of the relevant dipole-allowed transitions of HeHHe<sup>+</sup> outside a cavity, as determined from a time-independent NEO-CASCI calculation, color coded to match the relevant state from the middle panels.

## S2 HCN Vibronic Strong Coupling

We have additionally investigated vibronic strong coupling with the HCN molecule. The HCN geometry has a C–N distance of 1.15824 Å. The quantized proton basis functions and associated electronic basis functions are centered 1.0702 Å from the central carbon. We use the cc-pVDZ<sup>1</sup> electronic basis and PB4-D<sup>2</sup> protonic basis. The electronic active space is 2 electrons in 2 orbitals, which are described as the nitrogen lone pair orbital and the C–H  $\sigma^*$  antibonding orbital. The proton active space is 1 proton in 9 orbitals, including only those of s and p character along the C–H bonding axis. For real-time simulations, we utilize a timestep of 0.001 a.u. and propagate trajectories for a total time of 6000 a.u. All signal processing is performed using Fourier transforms (as opposed to the Padé approximants in the main text), with dampening factors of  $\tau = 0.8 \times 10^{-3}$  a.u. when calculating spectra and  $\tau = 1.0 \times 10^{-3}$  a.u. for taking the Fourier transform of the field displacement and projected coefficients.

We utilize the same three values of light matter coupling as used in the main text and tune the cavity to be resonant with the  $S_0\nu_0 \rightarrow S_1\nu_0$ ,  $S_0\nu_0 \rightarrow S_1\nu_1$ , and  $S_0\nu_0 \rightarrow S_1\nu_2$  molecular transitions. Calculated spectra, analogous to Figure 3 in the main text, are shown in Figure S2. Analyses of the polaritonic states, analogous to Figures 4 and 5 in the main text, are shown in Figures S3 and S4.

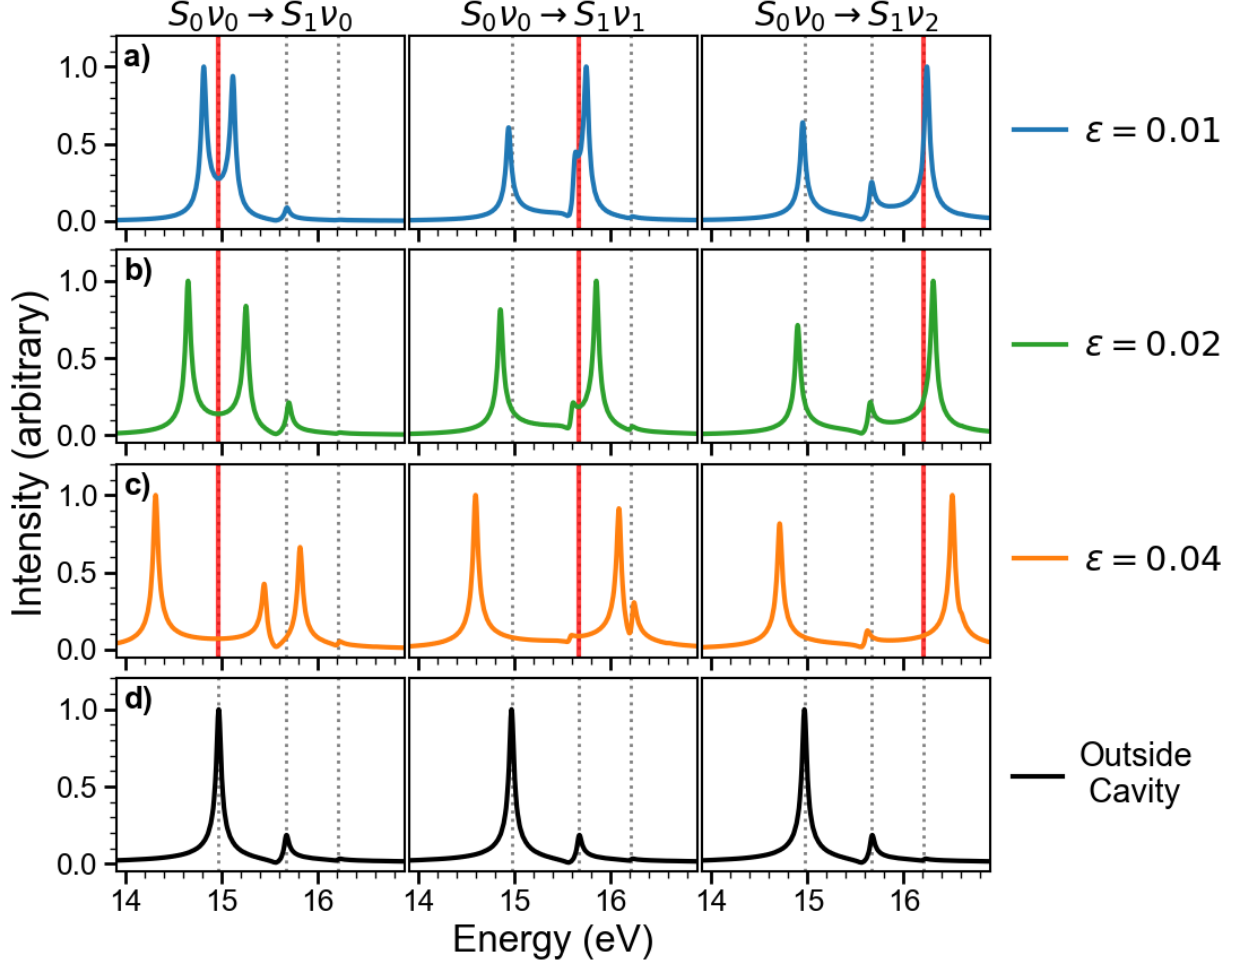

Figure S2: Spectra of HCN calculated using the semiclassical NEO-TDCI method with three different cavity mode frequencies and three different light-matter coupling strengths, compared to the spectrum outside the cavity. The cavity mode frequency is indicated at the top of each column and is shown as a solid red line on the plots. The light-matter coupling strength is indicated on the right of each row and increases from (a) 0.01 a.u. to (b) 0.02 a.u. to (c) 0.04 a.u. (d) Spectrum of HCN calculated outside the cavity. All plots in this row are identical, and the dotted vertical lines indicate the energies of the relevant dipole-allowed transitions of HCN outside the cavity, as determined from a time-independent NEO-CASCI calculation.

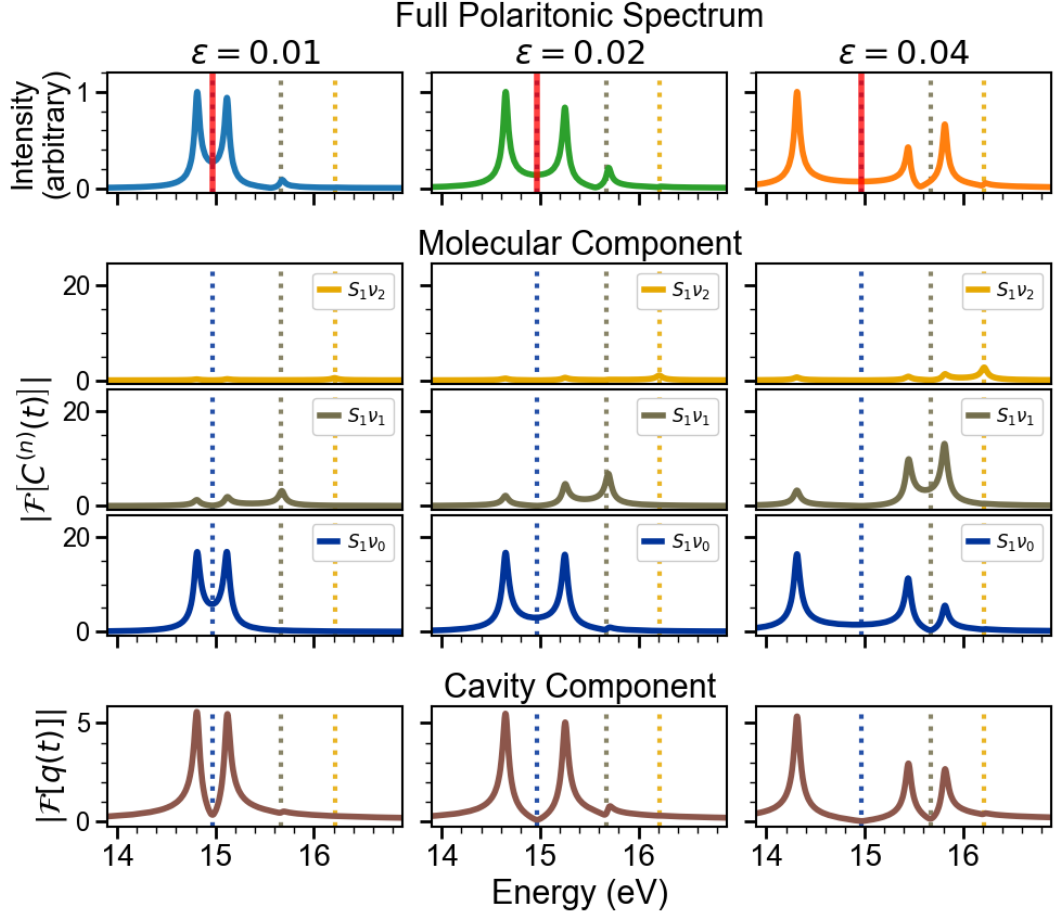

Figure S3: Top row: Semiclassical NEO-TDCI spectra of HCN calculated with the cavity mode frequency tuned to the  $S_0\nu_0 \rightarrow S_1\nu_0$  transition (solid red lines) and the light-matter coupling constant indicated above each column. Middle set of plots: Fourier transforms of the projected coefficients of the relevant molecular vibronic states for the light-matter coupling constants indicated above each column. Bottom row: Fourier transforms of the classical cavity mode displacement coordinate. On all plots, the dotted vertical lines indicate the energies of the relevant dipole-allowed transitions of HCN outside the cavity, as determined from a time-independent NEO-CASCI calculation, color coded to match the relevant state from the middle panels.

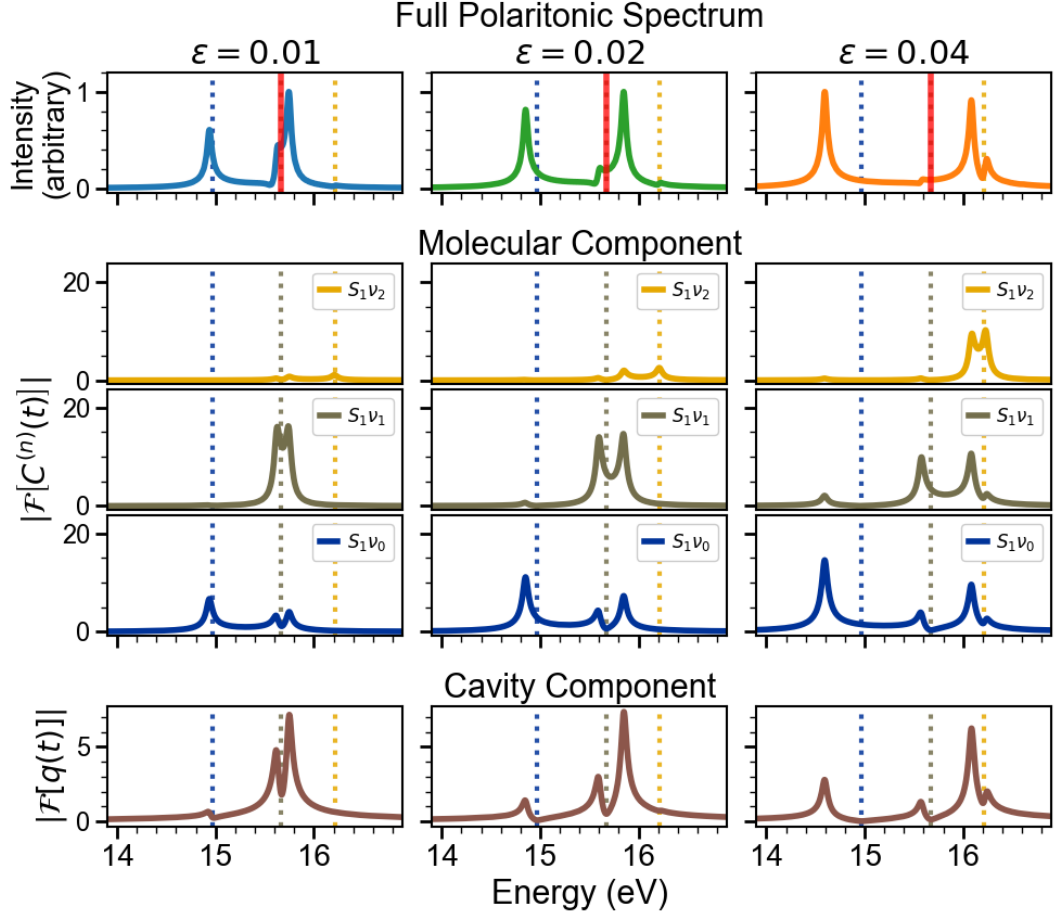

Figure S4: Top row: Semiclassical NEO-TDCI spectra of HCN calculated with the cavity mode frequency tuned to the  $S_0\nu_0 \rightarrow S_1\nu_1$  transition (solid red lines) and the light-matter coupling constant indicated above each column. Middle set of plots: Fourier transforms of the projected coefficients of the relevant molecular vibronic states for the light-matter coupling constants indicated above each column. Bottom row: Fourier transforms of the classical cavity mode displacement coordinate. On all plots, the dotted vertical lines indicate the energies of the relevant dipole-allowed transitions of HCN outside the cavity, as determined from a time-independent NEO-CASCI calculation, color coded to match the relevant state from the middle panels.

## References

- <sup>1</sup>T. H. Dunning Jr, “Gaussian basis sets for use in correlated molecular calculations. i. the atoms boron through neon and hydrogen”, J. Chem. Phys. **90**, 1007–1023 (1989).
- <sup>2</sup>Q. Yu, F. Pavošević, and S. Hammes-Schiffer, “Development of nuclear basis sets for multicomponent quantum chemistry methods”, J. Chem. Phys. **152**, 244123 (2020).
